# Supplementary material for: PartIR: Composing SPMD Partitioning Strategies for Machine Learning
Source: arXiv:2401.11202 source file (2024-11-24)
Supplement: Supplementary file 1 [file communication.tex]

\section{Communication optimizations}\label{sec:communication_extneded}
By virtue of our translation in
Figure~\ref{fig:Core-to-SPMD-translation} (cf. \Cref{thm:top-level-translation}) 
a \partir:Core program and its \partir:SPMD translation have the same
fully replicated tensor type.
The same is true for any top-level \coreloop and its translation.
This in turns means that an \spmdexecute takes as arguments replicated tensors even if the producer of these tensors is
another \spmdexecute operation that produces {\em distributed}
tensors. 
% a
% \partir:Core \coreloop translated in a context with
% stacked axes will be lowered to
% an \inlc{spmd.execute} operation that accepts
% replicated types in the same stacked context.
% \nrink{Needs rephrasing.}
% This in turns means that the translation of a top-level \coreloop
% operation takes as arguments fully replicated tensors, 
% even if the producer of these tensors is
% another \inlc{spmd.execute} operation that produces {\em distributed}
% tensors! 
In this section we outline communication optimizations that include removal of excessive replication.
%
% and similarly the \inlc{@main}
% function 
% program and its translation to \partir:SPMD
% have the same fully replicated type. 
%
% By \Cref{thm:top-level-translation}, a \partir:Core program $e$ and its translation $e'$ to \partir:SPMD have the same, fully replicated tensor type.
% Superficially, therefore, the translation to \partir:SPMD has not brought us any closer to a device-local computation on partitioned tensors.
% We now describe a number of transformations that are enabled by \partir:SPMD and that reduce the per-device memory consumption of device-local computations.
%
As a result,
function signatures and \inlc{spmd.execute} arguments are rewritten to accept distributed types, and
additional \spmdredist{s} appear.
We also briefly discuss how 
\spmdredist can be implemented using MPI-style collective operations.

\subsection{Optimizing per-device memory consumption}

% Device-local computations consume less memory than their global counterparts if tensors are genuinely distributed, i.e. if the device-local portions of a tensor is genuinely smaller than the full global tensor.
% The following two transformations therefore {\em genuinely} distribute the arguments of \spmdexecute instruction and function arguments.

\subsubsection{Transformation: distributing arguments of \spmdexecute instructions}
\label{sec:distributing-arguments}
We demonstrate this transformation with an example.
Consider an excerpt of the \inlc{spmd.execute} from \Cref{lst:SPMD-tiled-chain-matmul}:%
\begin{lstlisting}[language=mlir]
func @main(%x: dtensor<{}, [256,8]>, %w1: dtensor<{}, [8,16]>, ...) -> ... {
    %x1s0 = spmd.execute "a" ((*@\codehl{pink}{\%x}@*), %w1)
                (%ra: range<4>, %yx: tensor<256x8xf32>, %yw1: tensor<8x16xf32>) {
        (*@\codehl{pink}{\%xs  = slice 0 \%yx[\%ra]   : tensor<64x8xf32>} @*)
        ...
    } : dtensor<"a", [64,16]>
    ...
\end{lstlisting}
% \begin{lstlisting}[language=mlir]
% func @main(%x: dtensor<{}, [256,8]>, %w1: dtensor<{}, [8,16]>, %w2: dtensor<{}, [16,8]>)
%   -> dtensor<{}, [256,8]> attributes {mesh = {"a":4, "b":2}} {
%     %x1s0 = spmd.execute "a" ((*@\codehl{pink}{\%x}@*), %w1)
%                 (%ra: range<4>, %yx: tensor<256x8xf32>, %yw1: tensor<8x16xf32>) {
%         (*@\codehl{pink}{\%xs  = slice 0 \%yx[\%ra]   : tensor<64x8xf32>} @*)
%         %x1s = matmul(%xs,  %yw1) : tensor<64x16xf32>
%         yield %x1s : tensor<64x16xf32>
%     } : dtensor<"a", [64,16]>
%     ...
% \end{lstlisting}
The local variable \inlc{\%yx} is sliced 
with \inlc{slice 0 \%yx[\%ra]}, so it is wasteful 
to pass the full tensor \inlc{\%x} into the 
\inlc{spmd.execute} operation. In order to only pass a
local chunk,
we insert a redistribution, 
replace the argument of \spmdexecute,
and remove the \coreslice instruction:
% When a local variable $y$ is used inside the body of an \spmdexecute instruction only to be sliced, i.e. only in identical instructions \slice{d}{y}{r_a}, then there is no need to pass the full tensor $y$ to the \spmdexecute instruction.
% Instead, passing a local chunk of $y$ -- specifically the chunk sliced out by \slice{d}{y}{r_a} -- is sufficient for performing the computation in the body of the \spmdexecute instruction.
% In order to pass a local chunk only, the external argument of the \spmdexecute instruction that corresponds to $y$ must be distributed along dimension $d$ and across axis $a$.
% The \slice{d}{y}{r_a} instructions in the body of the \spmdexecute instruction must then be eliminated.
%
% As an example of this transformation, consider \Cref{lst:SPMD-tiled-chain-matmul}.
% The \coreslice instructions that consume local variables \inlc{\%yx}, \inlc{\%yx1s0} and \inlc{\%yw2} trigger the outlined optimizations, introducing three \spmdredist instructions, as sketched in the following code snippet.
\begin{lstlisting}[language=mlir]
func @main(%x: dtensor<{}, [256,8]>, %w1: dtensor<{}, [8,16]>, ...) -> ... {
    (*@\codehl{pink}{\%xd = spmd.redistribute \%x -> dtensor<\{\}, [\{"a"\}256,8]>} @*)
    %x1s0 = spmd.execute "a" ((*@\codehl{pink}{\%xd}@*), %w1)
                (%ra: range<4>, (*@\codehl{pink}{\%xs}@*): tensor<64x8xf32>, %yw1: tensor<8x16xf32>) {
          ...
    } : dtensor<"a", [64,16]>
    ...
\end{lstlisting}
Of course, this transformation only applies if \inlc{\%x} is not already partitioned along mesh axis \inlc{"a"}.
% \nrink{``partitioned'' or ``sharded''?
%     We seem to be using `sharded'' only once, when starting to discuss distributed types.
%     Is it worth having this terminology and risking confusing the reader?
% }
% \begin{lstlisting}[language=mlir]
% func @main(%x: dtensor<{}, [256,8]>, %w1: dtensor<{}, [8,16]>, %w2: dtensor<{}, [16,8]>)
%   -> dtensor<{}, [256,8]> attributes {mesh = {"a":4, "b":2}} {
%     (*@\codehl{pink}{\%xd = spmd.redistribute \%x -> dtensor<\{\}, [\{"a"\}256,8]>} @*)
%     %x1s0 = spmd.execute "a" ((*@\codehl{pink}{\%xd}@*), %w1)
%                 (%ra: range<4>, %yx: tensor<64x8xf32>, %yw1: tensor<8x16xf32>) {
%         %x1s = matmul(%yx,  %yw1) : tensor<64x16xf32>
%         yield %x1s : tensor<64x16xf32>
%     } : dtensor<"a", [64,16]>
%     ...
% \end{lstlisting}

% Importantly, this transformation has reduced the memory footprint of device-local computations since the local tensors passed into the bodies of the \spmdexecute instructions have become smaller.
% However, the \inlc{@main} function still consumes and produces fully replicated tensors.
% To address this, the next transformation propagates the \spmdredist instructions to the function's signature.

\subsubsection{Transformation: distributing tensors in function signatures}
% We have inserted an explicit redistribute command for \inlc{\%x}.
% However, the \inlc{@main} function still consumes and produces fully replicated tensors.
% To address this,
If all uses of a function argument (or the definition of a return value)
are identical redistribution instructions%
\footnote{We could also allow more powerful variants of this, e.g. identifying the {\em most distributed}
type of all redistributed uses.}, such as for \inlc{\%x} in the previous listing,
then we convert the function signature itself to use
distributed types:
% (the listing only shows how the argument type for \inlc{\%x} is converted): % If a function argument $x$ has type $\mu_1$ and all its uses are in identical \redist{x}{\mu_2} instructions, then the function's signature can be changed to accept an argument $x$ of type $\mu_2$ instead, and the \redist{x}{\mu_2} instructions can be eliminated.
% Dually, if a function returns a value $z$ that is produced by a \redist{y}{\mu_3} instruction, the function body can be rewritten to return $y{:}\mu_4$, meaning that the function's signature must be changed to have return type $\mu_4$.

% In the running code example, arguments \inlc{\%x} and \inlc{\%w2} as well as the value returned from \inlc{@main} are amenable to this transformation, which then produces the following code.
\begin{lstlisting}[language=mlir]
func @main(%x: (*@\codehl{pink}{dtensor<\{\}, [\{"a"\}256,8]>}@*), ...) -> ... {
    %x1s0 = spmd.execute "a" 
                (%x: dtensor<{}, [{"a"}256,8]>, %w1: dtensor<{}, [8,16]>)
                (%ra: range<4>, %yx: tensor<64x8xf32>, %yw1: tensor<8x16xf32>) { ... }
    ... 
\end{lstlisting}
Note that this transformation changes the calling convention for \inlc{@main}, which might need to be accounted for externally. When the \inlc{@main} function is now executed on all devices in the mesh, in an SPMD fashion, each device operates on a different device-local chunk of the function argument \inlc{\%x}.

\subsection{Rewriting \spmdredist instructions}
\label{sec:merging-redistribution}
As the previous transformations introduce
new \inlc{spmd.redistribute} instructions, it becomes
beneficial to fuse chains of them. 
% we implement rewrites \nrink{Just one, no?} that attempt to create \nrink{find?}
% chains of \spmdredist instructions and fuse them.
% Fusing of chains of redistributions is given by the following rewrite:
% programs we need to find ways to fuse them, since
%
%
% program we start seeing chains of redistributions
% that can easily be fused to a single one since
% redistribution does not modify the global denotations.
% We implement such optimizations that 
% Concretely we implement the follwing rewrite rule:
%
% The previous code example has a remaining \inlc{spmd.redistribute \%x1s0}, which redistributes between intermediate variables that are neither function arguments nor return values.
% When there are sequences of \spmdredist instructions, these can potentially be merged, as we now explain.
%
% \subsubsection{Transformation: merging redistributions}
% Pairs of \spmdredist instructions can be merged into a single \spmdredist instruction, i.e.
\[\footnotesize\begin{array}{rcl}
\begin{array}{l}
\plet y = \redist{x}{\mu_1} \pin e\\
\plet z = \redist{y}{\mu_2} \pin e
\end{array} &
    \rightsquigarrow &
\plet z = \redist{x}{\mu_2} \pin e
\end{array}\]%
The rewrite is valid because redistribution does not modify
the global tensor data. 

Additionally, any $\redist{x}{\mu}$ for $x{:}\mu$ is a trivial operation and we therefore eliminate it.
These trivial redistributions can occur as the result of previous fusions, for example.

%\apaszke{Note that sometimes \spmdredist commutes with \spmdtst.}
We also note that sometimes \spmdredist and $\tst{[\tileaction{a}{d}]}{}$ instructions commute.
This is the case, in particular, when the lowering from \Cref{fig:Core-to-SPMD-translation} invokes 
$\sigma \sfixup z \Downarrow \mu \rightsquigarrow \ldots$ multiple times at the end of a perfect loop nest.
The emitted instruction sequence consists of pairs of \spmdredist and \spmdtst instructions such that the \spmdredist instruction from one pair commutes with the \spmdtst instruction from the next pair.
Our implementation takes advantage of this commuting to expose additional opportunities for merging \spmdredist instructions.

% \noindent
% provided that $y$ on the left-hand side has no uses other than in the definition of $z$.
% No further code analysis is required to validate this rewrite:
% if the pair of \spmdredist instructions on the left is well-typed, so is the single \spmdredist instructions on the right.
% This is because the data equivalence relation $\sim$ in \Cref{fig:partir:spmd} is transitive.
%
% This rewriting of pairs of \spmdredist instructions extends to whole sequences that can then be collapsed into a single \spmdredist instruction
% (provided none of the intermediate values have other uses).
% This transformation is beneficial in the light of our lowering of \spmdredist instructions (see below):
% every \spmdredist instruction is lowered in isolation and results in at least one primitive for collective communication.
% Hence, fewer \spmdredist instructions may mean less communication.
% % it certainly means lower communication latency since fewer primitives means fewer program points at which communication must be initiated.

\ifextended
\else
Moreover, we often find
redistribution interspersed with other instructions
like \inlc{spmd.tile_reduce}. We can apply simple
reordering rewrites like the following:
% Note that sequences of \spmdredist instructions commonly arise as a result of repeatedly distributing the arguments of an \spmdexecute instruction.
% If an argument of an \spmdexecute instruction is sliced repeatedly inside the \spmdexecute instruction's body, these \coreslice instructions can successively be transformed into \spmdredist instructions outside of the \spmdexecute instruction, as explained above.
%
% \subsubsection{Transformation: reordering \coretile actions and \spmdredist instructions}
% When lowering nested \partir:Core \coreloop instructions with \coretile actions, the translation from \Cref{fig:Core-to-SPMD-translation} produces sequences of alternating \spmdtst and \spmdredist instructions.
% The \spmdtst instructions in these alternating sequences act as a blocker to merging of \spmdredist instructions.
% Thankfully, the alternating sequences produced by our translation can be reordered, and the \spmdredist instructions can simultaneously be merged, as specified by the rewrite rule
\[\footnotesize\begin{array}{l}
\begin{array}{l}
%\;\plet y_0 = \tst{[\tileaction{a_0}{d_0}]}{x_0} \\
\plet x_1 = \redist{y_0}{\mu_1} \;\pin \\
\plet y_1 = \tst{[\sigma]}{x_1}\;\pin \\
\plet x_2 = \redist{y_1}{\mu_2} \pin e
\end{array}
\rightsquigarrow
\begin{array}{l}
%\;\plet y_0 = \tst{[\tileaction{a_0}{d_0}]}{x_0} \\
\plet y_1 = \tst{[\sigma]}{y_0}\;\pin \\
\plet x_1 = \redist{y_1}{\tilered{\sigma}{\mu_1}}\;\pin \\
\plet x_2 = \redist{x_1}{\mu_2} \pin e
\end{array}
\end{array}\]
This rewrite is commuting the middle
\inlc{spmd.redistribute} and \inlc{spmd.tile_reduce}
instructions, which is always correct because 
because redistribution cannot affect the stacked axis
context of a type. The purpose of this reordering is
to later on enable fusion of $x_1$ and $x_2$. Note too, how
the $\mu_1$ type has to slightly be modified in the RHS 
to take the preceding action into account ($\tilered{\sigma}{\mu_1}$).
\dvytin{Norman, PTAL}
\nrink{The rewrite is not valid in general. It works when the \spmdredist are in fact \spmdallgather, but not for \spmdallslice?}
\fi

% Note that this rigid relation between the types $\mu_0, \mu_1, \mu_2$ holds because we assume that the sequence of instructions on the left-hand side of the rewrite rule was obtained from lowering nested \partir:Core \coreloop instructions.

\subsection{Lowering redistribution and \spmdtst instructions}

Redistribution generally requires communication, so we ultimately lower \spmdredist instructions to sequences of MHLO's MPI-style primitives for collective communication \cite{xla, mpi}.
In doing so, we use versions of these primitives that carry mesh axes as static attributes.
These attributes specify communication patterns at a higher level of abstraction than device ids (or {\em ranks} in MPI parlance), and they align well with our distributed types by admitting typing rules such as the following for \spmdallgather:%
\footnote{Syntax and typing rule for the full set of \partir:SPMD primitives for collective communication are given in \Cref{app:sec:collective-communication}.}
\begin{mathpar}\footnotesize
  \Infer{TAllGather}
        { \Gamma \tspmd x : \disttensor{\cs}{[\{\as_1\bs_1\}n_1,\ldots,\{\as_k\bs_k\}n_k]} }
        { \Gamma \tspmd \allgather{[\as_1, \ldots, \as_k]}{x} : \disttensor{\cs}{[\{\bs_1\}n_1,\ldots,\{\bs_k\}n_k]} }
\end{mathpar}

While \cite{redist2021} gives a general method for efficiently implementing redistribution, in \partir we have found the following to work sufficiently well in practice.
Given types
{\small\begin{gather*}
    \mu_1 = \disttensor{\cs_{\textit stacked}}{[\{\as_1\cs_1\}n_1,\ldots,\{\as_k\cs_k\}n_k]}
    \,, \\
    \mu_2 = \disttensor{\cs_{\textit stacked}}{[\{\bs_1\cs_1\}n_1,\ldots,\{\bs_k\cs_k\}n_k]}
    \,,
\end{gather*}}%
we implement \redist{x}{\mu_2} for $x$ of type $\mu_1$ as
{\small\begin{gather*}
    \plet x''{:}\mu'' = \allgather{[\as_1,\ldots,\as_k]}{x} \pin
    \allslice{[\bs_1,\ldots,\bs_k]}{x'} \,,
\end{gather*}}%
where $\mu'' = \disttensor{\cs_{\textit stacked}}{[\{\cs_1\}n_1,\ldots,\{\cs_k\}n_k]}$,
and \spmdallslice has a typing rule dual to \textsc{TAllGather}.
Syntactically, one regards $\mu''$ as a common suffix type of $\mu_1$ and $\mu_2$.
Semantically, this means that the intermediate tensor $x''$ is only as replicated as it needs to be to enable an implementation of \redist{x}{\mu_2}
with a single pair of \spmdallgather and \spmdallslice.
% \nrink{The previous two sentences can be removed, but given that this section already skips a lot of detail, it adds a bit of nice intuition that might help the reader follow along.}

A \tst{[\sumaction{a}]}{x} also requires communication, and it lowers to \spmdallsum:
\begin{mathpar}\footnotesize
  \Infer{TAllSum}
        { \Gamma \tspmd x : \disttensor{\cs a}{[\{\bs_1\}n_1,\ldots,\{\bs_k\}n_k]} }
        { \Gamma \tspmd \allsum{a}{x} : \disttensor{\cs}{[\{\bs_1\}n_1,\ldots,\{\bs_k\}n_k]} }
\end{mathpar}
A \tst{[\tileaction{a}{d}]}{x}, on the other hand, is a trivial operation:
it only changes the type of $x$ to specify how the local tensors stacked along axis $a$ are to be viewed as a global tensor.

\ifextended
\else
The \spmdredist instruction generally requires communication across devices to facilitate redistribution of its tensor argument.
Ultimately we implement this communication with XLA's primitives for collective communication \cite{Reference!}, which are analogous to MPI's communication primitives \cite{Reference!}.
However, a wide abstraction gap needs to be bridged by this implementation:
\spmdredist instructions specify communication at a are very high abstraction level, mentioning only the final distributed types, whereas XLA/MPI-style primitives are very low-level, operating in terms of device ids (or {\em ranks}, in MPI parlance).

We bridge this gap by adding to \partir:SPMD the four communication primitives that are introduced by \Cref{fig:partir:spmd-communication-primitives}.
These primitives carry lists of axes (or, in the case of \spmdallsum, a single list of axes) as static attributes,
and these list specify the communication pattern for each specific instance of a communication primitives.
By virtue of the typing rules in \Cref{fig:partir:spmd-communication-primitives}, the axes attributes are firmly tied to the argument and result types of a communication primitive.
This makes it easy to lower \spmdredist instructions to sequences of the primitives in \Cref{fig:partir:spmd-communication-primitives}.
At the same time, the axis attributes -- in the presence of a statically fixed mesh $M$ -- allow us to compute statically the device ids that need to be passed to the XLA counterpart of each of the \partir:SPMD communication primitives.

We now explain how we implement a \spmdredist instruction in terms of \spmdallgather and \spmdallslice primitives.
Consider the types
%%
% \begin{align*}
% &    \mu_1 = \disttensor{\cs_{\textit stacked}}{[\{\as_1\cs_1\}n_1,\ldots,\{\as_k\cs_k\}n_k]} \,,
%      \,\, \text{and} \\
% &    \mu_2 = \disttensor{\cs_{\textit stacked}}{[\{\bs_1\cs_1\}n_1,\ldots,\{\bs_k\cs_k\}n_k]} \,,
% \end{align*}
{\small\begin{gather*}
\mu_1 = \disttensor{\cs_{\textit stacked}}{[\{\as_1\cs_1\}n_1,\ldots,\{\as_k\cs_k\}n_k]}
     ~ \text{and} ~
\mu_2 = \disttensor{\cs_{\textit stacked}}{[\{\bs_1\cs_1\}n_1,\ldots,\{\bs_k\cs_k\}n_k]}
\end{gather*}}

\noindent
which satisfy $\mu_1 \sim \mu_2$.
Assume we are given $x{:}\mu_1$ and need to implement \redist{x}{\mu_2}.
This can always be achieved with a single pair of \spmdallgather and \spmdallslice:
%%
% \begin{align*}
% &    \plet x'{:}\mu' = \spmdallgather{\,[\as_1\cs_1,\ldots,\as_k\cs_k]\,}{x} \pin \\
% &    \spmdallslice{\,[\bs_1\cs_1,\ldots,\bs_k\cs_k]\,}{x'}
%      \,,
% \end{align*}
{\small\begin{gather*}
\plet x'{:}\mu' = \spmdallgather{\,[\as_1\cs_1,\ldots,\as_k\cs_k]\,}{x} \pin \spmdallslice{\,[\bs_1\cs_1,\ldots,\bs_k\cs_k]\,}{x'}
     \,,
\end{gather*}}

\noindent
where $\mu' = \disttensor{\cs_{\textit stacked}}{[n_1,\ldots,n_k]}$.
Hence the intermediate tensor $x'$ is fully replicated, which is why the above pair of \spmdallgather and \spmdallslice is in fact the least memory-efficient way of implementing \redist{x}{\mu_2}.

A general method for implementing redistribution in a memory-efficient way, while also aiming to minimize data transfers, appears in \cite{redist2021}.
In our implementation of \partir, we have found the following improvement over the pair of \spmdallgather and \spmdallslice above to work sufficiently well in practice:
%%
% {\footnotesize
% \begin{align*}
% &    \plet x''{:}\mu'' = \spmdallgather{\,[\as_1,\ldots,\as_k]\,}{x} \pin \\
% &    \spmdallslice{\,[\bs_1,\ldots,\bs_k]\,}{x'}
%      \,,
% \end{align*}
% }
{\small\begin{gather*}
    \plet x''{:}\mu'' = \spmdallgather{\,[\as_1,\ldots,\as_k]\,}{x} \pin
    \spmdallslice{\,[\bs_1,\ldots,\bs_k]\,}{x'} ~,
\end{gather*}}

\noindent
where $\mu'' = \disttensor{\cs_{\textit stacked}}{[\{\cs_1\}n_1,\ldots,\{\cs_k\}n_k]}$.
Syntactically, one regards $\mu''$ as a common suffix type of $\mu_1$ and $\mu_2$.
Semantically, this means that the intermediate tensor $x''$ is only as replicated is it needs to be to enable an implementation of \redist{x}{\mu_2}
with a single pair of \spmdallgather and \spmdallslice.

Note that if $\mu'' = \mu_1$ or $\mu'' = \mu_2$, one only needs either the \spmdallslice instruction or the \spmdallgather instruction to implement \redist{x}{\mu_2};
and, of course, if $\mu_1 = \mu_2$, then \redist{x}{\mu_2} is a trivial operation that can be eliminated, and hence requires no communication.
In the general case then, every \redist{x}{\mu_2} is implemented with at least one communication primitive, which is why it is beneficial to first merge sequences of \spmdredist instructions into as few as possible, as described in \Cref{sec:merging-redistribution}.

\begin{figure}[t]\footnotesize
\[\begin{array}{ll}
    \begin{array}{lcl}
        \multicolumn{3}{l}{\textbf{Value definitions}} \\
        v &  ::= & \ldots \quad\text{(\partir:SPMD instructions from \Cref{fig:partir:spmd})} ~\mid~
                   \allgather{[\as_1, \ldots, \as_k]}{x} \\
          & \mid & \allsum{\as}{x}                       ~\mid~
                   \allslice{[\as_1, \ldots, \as_k]}{x}  ~\mid~
                   \sumscatter{[\as_1, \ldots, \as_k]}{x}   
    \end{array} &
\end{array}\]
~\\
\text{{\bf Typing} (in the presence of an implicitly given mesh $M$ that binds all axis identifiers mentioned in the rules)}
\begin{mathpar}
  \Infer{TAllGather}
        { \Gamma \tspmd x : \disttensor{\cs}{[\{\as_1\bs_1\}n_1,\ldots,\{\as_k\bs_k\}n_k]} }
        { \Gamma \tspmd \allgather{[\as_1, \ldots, \as_k]}{x} : \disttensor{\cs}{[\{\bs_1\}n_1,\ldots,\{\bs_k\}n_k]} } \\ 
  \Infer{TAllSum}
        { \Gamma \tspmd x : \disttensor{\cs}{[\{\bs_1\}n_1,\ldots,\{\bs_k\}n_k]} \qquad
           \set{\cs} = \set{\as} \cup \set{\cs'} }
        { \Gamma \tspmd \allsum{\as}{x} : \disttensor{\cs'}{[\{\bs_1\}n_1,\ldots,\{\bs_k\}n_k]} } \\ 
  \Infer{TAllSlice}
        { \Gamma \tspmd x : \disttensor{\cs}{[\{\bs_1\}n_1,\ldots,\{\bs_k\}n_k]} }
        { \Gamma \tspmd \allslice{[\as_1, \ldots, \as_k]}{x} : \disttensor{\cs}{[\{\as_1\bs_1\}n_1,\ldots,\{\as_k\bs_k\}n_k]} } \\ 
  \Infer{TSumScatter}
        { \Gamma \tspmd x : \disttensor{\cs}{[\{\bs_1\}n_1,\ldots,\{\bs_k\}n_k]} \\
          \set{\cs} = \set{\as_1} \cup \cdots \cup \set{\as_k} \cup \set{\cs'} }
        { \Gamma \tspmd \sumscatter{[\as_1, \ldots, \as_k]}{x} : \disttensor{\cs'}{[\{\as_1\bs_1\}n_1,\ldots,\{\as_k\bs_k\}n_k]} }
\end{mathpar}
\caption{
    \partir:SPMD primitives for collective communication.
    \nrink{
        Please someone check this figure carefully!
        This looks so much simpler than \cite{redist2021}, so I am concerned this figure is missing something!
        (If nothing is missing, then all of the added complications in \cite{redist2021} must be due to tracking in the types also the local dimensions --
        and, of course, there is an {\tt all\_to\_all} operation in \cite{redist2021} too.)
    }
}
\label{fig:partir:spmd-communication-primitives}
\end{figure}

We conclude this section by noting that the typing rules in \Cref{fig:partir:spmd-communication-primitives} present a slight generalization of the signatures for communication primitives that appear in \cite{redist2021}.
We include stacked axes in our presentation since they are operated on by the \spmdallsum and \spmdsumscatter instructions
(while being preserved by \spmdallgather and \spmdallslice).
The need to include primitives for collective summation is explained in the next section.
\fi

\subsection{Emitting device-local MHLO}

Assuming that all \spmdredist and \spmdtst instructions in a \partir:SPMD program have been lowered to communication primitives, it is straightforward to convert the program to a device-local MHLO computation in four steps:
\begin{enumerate}
    \item \label{mhlo-emission-step-1}
    Convert the distributed tensor types of all function arguments and top-level instructions to their corresponding local types.
    The communication primitives are converted into variants that accept and return local types instead of distributed types.
    \item \label{mhlo-emission-step-slice}
    Replace any \coreslice instructions remaining in \spmdexecute bodies by MHLO %\inlc{ReplicaId} and
    \inlc{DynamicSlice} operations.
    (The optimization from \Cref{sec:distributing-arguments} might fail to remove some \coreslice{s}.)
    \item \label{mhlo-emission-step-2}
    Eliminate \spmdexecute operations by inlining their bodies into the top block.
    % Hoist the code in the bodies of \spmdexecute instructions to the top level; then remove all \spmdexecute instructions (whose bodies are now empty).
    Note that all tensor types \spmdexecute bodies were already local prior to this inlining;
    % However, for the hoisting to produce valid top-level code, all local variables in the body of a given \spmdexecute instruction must be replaced with the corresponding external arguments of the \spmdexecute instruction.
    and no references to range variables remain in any \spmdexecute bodies after step \ref{mhlo-emission-step-slice}.
    \item \label{mhlo-emission-step-3}
    Convert any communication primitives to their MHLO XLA counterparts.
    This requires a conversion of axis names into MHLO-style replica groups~\cite{xla}.
    % This requires computing device ids from the axis attributes of communication primitives since the communication patterns for MHLO XLA primitives are specified in terms of device ids.
    % Note that MHLO XLA communication primitives accept and return local types, making the program well-typed again.
    % Hence, after converting to MHLO XLA primitives, the local types that were problematic in step \ref{mhlo-emission-step-1} are correct again.
\end{enumerate}
