# Supplementary material for: PartIR: Composing SPMD Partitioning Strategies for Machine Learning
Source: arXiv:2401.11202 source file (2024-11-24)
Supplement: Supplementary file 2 [file spmd_extended.tex]

\subsubsection{Simulation of global tensor types with distributed types}

The translation relation from \Cref{fig:Core-to-SPMD-translation} satisfies the following theorem, which states that when translating a \partir:Core expression $e$ of type \tensor{\ol{n}}, the resulting \partir:SPMD expression $e'$ has a distributed type that simulates \tensor{\ol{n}}. 
Moreover, the resulting distributed type \disttensor{\as}{\ol{n}} remembers the nesting level $\sigmas$ at which $e$ was defined, because $\as = \axes{\sigmas}$.

\begin{theorem}[Typing simulation]
\label{thm:top-level-translation}
Let $\Gamma \tcore \pctx{C}[e] : \tensor{\ol{n}}$ and let $\sigmas$ be such that $\axes{\sigmas} = a_1\cdots a_k$, where $r_{a_1},\ldots,r_{a_k}$ are the range variables in $\Gamma$.
If $\mathcal{M}$ satisfies
\begin{align*}
    \mapping{x{:}\tensor{\ol{m}}}{y{:}\disttensor{\bs}{\ol{m}}}{} \in \mathcal{M}
        \quad \Leftrightarrow \quad
    x{:}\tensor{\ol{m}}\in\Gamma
    \,\land\, 
    \ol{r_b} \text{ precede } x \text{ in }\Gamma
    \,,
\end{align*}
then there exists a (necessarily unique) $e'$ such that
\begin{itemize}
    \item $\mathcal{M}, \sigmas \vdash \langle \pctx{C}; e\rangle \rightsquigarrow e'$ and
    \item $\Gamma_{\mathcal{M}} \tspmd e' : \disttensor{a_1\cdots a_k}{\ol{n}}$,
\end{itemize}
where $\Gamma_{\mathcal{M}}$ contains precisely the pairs $y{:}\mu$ in the image of the map $\mathcal{M}$.
\end{theorem}
The proof of the theorem is standard and proceeds by structural induction on $e$.
The more interesting proof is the one that establishes correctness of the translation relation from \Cref{fig:Core-to-SPMD-translation}.
However, the statement of the corresponding correctness theorem requires additional machinery, specifically the definition of formal semantics for \partir:Core and \partir:SPMD.
We leave these technical details for \Cref{app:sec:translation-correctness}, stressing here only that we have indeed formally established the correctness of the translation defined by \Cref{fig:Core-to-SPMD-translation}.

\subsection{\partir:SPMD primitives for collective communication}
\label{app:sec:collective-communication}
Our \spmdredist instructions specify communication at a high abstraction level, mentioning only the final distributed types.
Contrast this with the lower-level MHLO's MPI-style primitives for collective communication that operate on device ids \cite{xla, mpi}.

To bridge the gap in abstraction levels, we add to \partir:SPMD the four communication primitives that are introduced by \Cref{fig:partir:spmd-communication-primitives}.
These primitives carry lists of axes (or, in the case of \spmdallsum, a single list of axes) as static attributes,
and these lists specify the communication pattern for each specific instance of a communication primitive.
By virtue of the typing rules in \Cref{fig:partir:spmd-communication-primitives}, the axes attributes are firmly tied to the argument and result types of a communication primitive.
This makes it easy to expand \spmdredist instructions into sequences of these primitives.
At the same time, the axis attributes -- in the presence of a statically fixed mesh $M$ -- allow us to compute statically the device ids that need to be passed to the MHLO XLA counterpart of each of the \partir:SPMD communication primitives.

\begin{figure}[t]\footnotesize
\[\begin{array}{ll}
    \begin{array}{lcl}
        \multicolumn{3}{l}{\textbf{Value definitions}} \\
        v &  ::= & \ldots \quad\text{(\partir:SPMD instructions from \Cref{fig:partir:spmd})} ~\mid~
                   \allgather{[\as_1, \ldots, \as_k]}{x} \\
          & \mid & \allsum{\as}{x}                       ~\mid~
                   \allslice{[\as_1, \ldots, \as_k]}{x}  ~\mid~
                   \sumscatter{[\as_1, \ldots, \as_k]}{x}   
    \end{array} &
\end{array}\]
~\\
\text{{\bf Typing} (in the presence of an implicitly given mesh $M$ that binds all axis identifiers mentioned in the rules)}
\begin{mathpar}
  \Infer{TAllGather}
        { \Gamma \tspmd x : \disttensor{\cs}{[\{\as_1\bs_1\}n_1,\ldots,\{\as_k\bs_k\}n_k]} }
        { \Gamma \tspmd \allgather{[\as_1, \ldots, \as_k]}{x} : \disttensor{\cs}{[\{\bs_1\}n_1,\ldots,\{\bs_k\}n_k]} } \\ 
  \Infer{TAllSum}
        { \Gamma \tspmd x : \disttensor{\cs}{[\{\bs_1\}n_1,\ldots,\{\bs_k\}n_k]} \qquad
           \set{\cs} = \set{\as} \cup \set{\cs'} }
        { \Gamma \tspmd \allsum{\as}{x} : \disttensor{\cs'}{[\{\bs_1\}n_1,\ldots,\{\bs_k\}n_k]} } \\ 
  \Infer{TAllSlice}
        { \Gamma \tspmd x : \disttensor{\cs}{[\{\bs_1\}n_1,\ldots,\{\bs_k\}n_k]} }
        { \Gamma \tspmd \allslice{[\as_1, \ldots, \as_k]}{x} : \disttensor{\cs}{[\{\as_1\bs_1\}n_1,\ldots,\{\as_k\bs_k\}n_k]} } \\ 
  \Infer{TSumScatter}
        { \Gamma \tspmd x : \disttensor{\cs}{[\{\bs_1\}n_1,\ldots,\{\bs_k\}n_k]} \\
          \set{\cs} = \set{\as_1} \cup \cdots \cup \set{\as_k} \cup \set{\cs'} }
        { \Gamma \tspmd \sumscatter{[\as_1, \ldots, \as_k]}{x} : \disttensor{\cs'}{[\{\as_1\bs_1\}n_1,\ldots,\{\as_k\bs_k\}n_k]} }
\end{mathpar}
\caption{
    \partir:SPMD primitives for collective communication.
    It is assumed that all $n_i$ in the distributed dimensions are evenly divisible by the product of axis sizes in that dimension.
}
\label{fig:partir:spmd-communication-primitives}
\end{figure}
We stress that including the \spmdsumscatter primitive in \partir:SPMD, in principle, enables fusion of \spmdallsum with \spmdallslice instructions.
Reasoning about when this kind of fusion can be applied and working out the details of how exactly it should be applied are facilitated by the axis attributes on the \partir:SPMD communication primitives.

The typing rules in \Cref{fig:partir:spmd-communication-primitives} present a slight generalization of the signatures for communication primitives in \cite{redist2021}:
we include stacked axes here since they are operated on by the \spmdallsum and \spmdsumscatter instructions (while being preserved by \spmdallgather and \spmdallslice).
